# Supplementary material for: StaticFixer: From Static Analysis to Static Repair
Source: arXiv:2307.12465 source file (2023-07-24)
Supplement: Supplementary file 1 [file appendix.tex]

%% Appendix
\appendix
\section{Appendix}

Text of appendix \ldots
